# Supplementary material for: RLlib Flow: Distributed Reinforcement Learning is a Dataflow Problem
Source: arXiv:2011.12719 source file (2021-10-28)
Supplement: Supplementary file 1 [file supplementary.tex]

\documentclass{article}
\input{packages}
\input{macros}

\usepackage{icml2021}

\begin{document}

\appendix
\renewcommand{\thesection}{A.\arabic{section}}
\renewcommand{\thefigure}{A\arabic{figure}}
\renewcommand{\thetable}{A\arabic{table}}
\setcounter{section}{0}
\setcounter{figure}{0}
\setcounter{table}{0}

\input{sections/appendix}

\end{document}
